# Supplementary material for: Primal Dual Affine Scaling on GPUs
Source: arXiv:1502.03543 source file (2015-02-12)
Supplement: Supplementary file 1 [file appendix.tex]

\subsection*{Simplifying the system of equations (\ref{eq:bigsystem})}
The following method was not found in any literature. Although no claim of originality is made here.
\begin{equation}
	\begin{bmatrix}
	A&O&O\\
	O&A^T&I\\
	S&O&X
	\end{bmatrix}\begin{bmatrix}
	\Delta x\\
	\Delta y\\
	\Delta s
	\end{bmatrix}=\begin{bmatrix}
	\vec{0}\\
	\vec{0}\\
	-X_ks^k
	\end{bmatrix}\nonumber
\end{equation}
First multiplying both sides by  $$I_{c1}=\begin{bmatrix}
I^{m+n\times m+n}&O^{m+n\times n}\\
O^{n\times n+m}&S^{-1}
\end{bmatrix}$$ gives the system 

\begin{equation}
	\begin{bmatrix}\label{eq:bigsystem3}
		A&O&O\\
		O &A^T&I \\
		I &O &S^{-1}X
		\end{bmatrix}\begin{bmatrix}
		\Delta x\\
		\Delta y\\
		\Delta s
		\end{bmatrix}=
		\begin{bmatrix}
		\vec{0}\\
		\vec{0}\\
		-\vec{x}
	\end{bmatrix}
\end{equation}
Now multiplying system (\ref{eq:bigsystem3}) with $$I_{c2}=\begin{bmatrix}
	O &I^{n\times n}&O\\
	I^{m\times m}&O &O\\
	O&O&I^{n\times n}
\end{bmatrix}$$ gives the system
\begin{equation}
	\begin{bmatrix}\label{eq:bigsystem4}
		O&A^T&I\\
		A&O&O\\
		I&O&S^{-1}X
	\end{bmatrix}
	\begin{bmatrix}
		\Delta x\\
		\Delta y\\
		\Delta s
	\end{bmatrix}=
	\begin{bmatrix}
		\vec{0}\\
		\vec{0}\\
		-\vec{x}
	\end{bmatrix}
\end{equation}

$$Z=
\begin{bmatrix}
	O&A^T&I\\
	A&O&O\\
	I&O&D
\end{bmatrix}
$$
$$
Z^{-1}=\begin{bmatrix}
	DA^TXAD-D&DA^T X &I-DA^T X A\\
	 X AD& X &- X A\\
	\left[I-DA^T X A\right]^T&-A^T X  &A^T X A
\end{bmatrix}$$
\hfill {\tiny $X=(ADA^T)^{-1}$}
$$
\begin{bmatrix}
	\Delta x\\
	\Delta y\\
	\Delta s
\end{bmatrix}=
\begin{bmatrix}
	-\left[I-DA^T(ADA^T)^{-1}A\right]\vec{x}\\
	 \left[(ADA^T)^{-1}A\right]\vec{x}\\
	-\left[A^T(ADA^T)^{-1}A\right]\vec{x}
\end{bmatrix}
$$
